# Supplementary material for: Pessimistic Model-based Offline Reinforcement Learning under Partial Coverage
Source: arXiv:2107.06226 source file (2023-01-10)
Supplement: Supplementary file 1 [file appendix.tex]

\section{Auxiliary Lemma}
\label{app:lemmas}

\begin{lemma}Consider any policy $\pi: \Scal\mapsto \Delta(\Acal)$, and denote $d^{\pi}$ as its state-action distribution. We have:
\begin{align*}
d^{\pi}(s,a) = (1 - \gamma) \mu_0(s) \pi(a|s) + \gamma \sum_{\tilde{s},\tilde{a}} d^{\pi}(\tilde{s},\tilde{a}) P(s | \tilde{s}, \tilde{a}) \pi(a|s).
\end{align*}
\end{lemma}
\begin{proof}
By definition, we have:
\begin{align*}
d^{\pi}(s,a) = & (1-\gamma) \sum_{h=0}^{\infty} \gamma^h d^{\pi}_h(s,a) = (1-\gamma) d^{\pi}_0(s,a) + (1-\gamma)  \sum_{h=1}^{\infty}  \gamma^h d^{\pi}_h(s,a) \\
& =  (1-\gamma) d^{\pi}_0(s,a) + (1-\gamma)  \sum_{h=1}^{\infty}  \gamma^h \sum_{\tilde{s},\tilde{a}}d^{\pi}_{h-1}(\tilde{s},\tilde{a}) P(s | \tilde{s},\tilde{a}) \pi(a|s)  \\
& = (1-\gamma) d^{\pi}_0(s,a) +  \gamma \sum_{\tilde{s},\tilde{a}} (1-\gamma) \sum_{h=0}^{\infty}   \gamma^h d^{\pi}_h(\tilde{s},\tilde{a}) P(s | \tilde{s},\tilde{a}) \pi(a|s) \\
& = (1-\gamma) d^{\pi}_0(s,a) +\gamma \sum_{\tilde{s},\tilde{a}} d^{\pi}(\tilde{s},\tilde{a}) P(s | \tilde{s},\tilde{a}) \pi(a|s)
\end{align*}
\end{proof}

\begin{lemma}[MLE guarantee] Given a set of models $\Mcal = \{ P: \Scal\times\Acal\mapsto \Delta(\Scal)\}$ with $P^\star \in \Mcal$, and a dataset $\Dcal = \{s_i,a_i, s'_i\}_{i=1}^N$ with $s_i,a_i \sim \rho$, and $s'_i\sim P^\star(s_i,a_i)$, denote $\widehat{P}_{mle}$ as the MLE $$ \widehat{P}_{mle} = \argmin_{P\in\Mcal} \sum_{i=1}^N - \ln P(s_i' | s_i,a_i). $$ With probability at least $1-\delta$, we must have:
\begin{align*}
\mathbb{E}_{s,a\sim \rho} \left\| \widehat{P}_{mle}(\cdot |s,a) - P^\star(\cdot | s,a)  \right\|_1^2 \leq \frac{ \ln(|\Mcal| / \delta) }{N}.
\end{align*}
\end{lemma}
For proof, we refer readers to Flambe.
